# Supplementary material for: Are Akpans Trick or Treat: Unveiling Helpful Biases in Assistant Systems
Source: arXiv:2205.12554 source file (2025-03-02)
Supplement: Supplementary file 1 [file 2-heuristics.tex]

\section{Heuristics for Filtering Classifier}
