# Supplementary material for: Are Akpans Trick or Treat: Unveiling Helpful Biases in Assistant Systems
Source: arXiv:2205.12554 source file (2025-03-02)
Supplement: Supplementary file 2 [file 5-error-analysis.tex]

% We will provide a more thorough error analysis together with examples in the appendix. AppendixC provides the spurious correlation of easy patterns that our earlier models captured to make decisions in the dataset.
