# Supplementary material for: Are Akpans Trick or Treat: Unveiling Helpful Biases in Assistant Systems
Source: arXiv:2205.12554 source file (2025-03-02)
Supplement: Supplementary file 3 [file _1-statistics.tex]

\section{Statistics for Collected }
